# Supplementary material for: Cooperative Infrastructure Perception
Source: arXiv:2207.08930 source file (2024-06-26)
Supplement: Supplementary file 1 [file appendix.tex]

\newpage
\appendix
\section*{Appendix}
\label{sec:appendix}

\section{Finding Initial Guesses for Alignment}
\label{s:find-init-guess}

\parab{Overview.}  In this section, we detail the proposed method (\algoref{algo:icp}) to find good initial guesses for ICP based alignment in \sysname with \emph{minimal information}. The input to the proposed algorithm (Algorithm \ref{algo:icp}) is a set of $N > 1$ point clouds, $\mathbf{C} = \{ C_1, C_2, \cdots, C_N\}$, from a set of roadside LiDARs, $\mathbf{L} = \{ L_1, L_2, \cdots, L_N\}$, and the ground distances between every LiDAR ($L_i$) and a \emph{reference} LiDAR (say, $L_1$):  $d_{i}$ (we can obtain the distance between any pair of LiDAR's by using an off-the self laser range finders). The output of the algorithm is a set of transformation matrices between a LiDAR's coordinate system and the \emph{reference} LiDAR's coordinate system. 
% The proposed algorithm has three main components: (1) Ground Plane segmentation and Ground Plane Alignment, (2) Position Alignment, and (3) Yaw Estimation

\parab{Estimating Position, Roll and Pitch.} Assuming the \textit{ground-plane} is the largest visible plane with significant visibility overlaps for every pair of LiDARs in \sysname (a reasonable assumption for roadside LiDARs), we, first, perform a ground plane segmentation in every point cloud $C_i$ (\algolineref{algo:icp}{icp:ln3}) using fast \textit{plane-finding} algorithms~\cite{derpanis2010overview}. 
Next, we align the ground plane of each LiDAR ($L_i$) with the ground plane of the reference LiDAR ($L_0$) with the known distance $d_{i1}$ to get an initial estimate of the respective LiDAR's roll (angle around the $x$ axis) and pitch (angle around the $x$ axis). To this, we set \emph{reference} LiDAR $L_1$'s $x$ and $y$ coordinates to be $(0,0)$ (\ie the base of the LiDAR is at the origin). Now for every LiDAR $L_i$ we only consider the relative position; using the known distance $d_i$ we say $L_i$'s base is at $(d_i,0)$ and perform the alignment (\algolinesref{algo:icp}{icp:ln4}{icp:ln5}). We use the aligned point clouds to also get the height of each LiDAR $z_i$ which is the LiDAR's location along the normal to the ground plane. At this point, the only thing that remains is to determine the yaw (angle around the $z$ axis) of the LiDARs $L_i$ and $L_1$.

\begin{algorithm}
\SetAlgoLined
\SetKwInOut{Input}{input}
\SetKwInOut{Output}{output}
\SetKw{KwBy}{by}

\Input{(1) A set of Point Clouds, $\mathbf{C} = \{C_1,  \cdots, C_N\}$, where $C_i$ denotes the Point Cloud of LiDAR $L_i$. \newline
(2) A set of distances from the reference LiDAR, $D = \{d_2, \cdots, d_N\}$, where $d_i$ is the known distance from LiDAR $i$ to LiDAR 1.
}
\Output{A set of transformations $T = \{T_2, T_3, \cdots, T_N\}$; we can apply transformation $T_i$ to point cloud $C_i$ to translate into the \emph{reference} LIDAR's ($C_1$) coordinate system.}

Ground Plane Segmentation of $C_1$

\For{$i\gets2$ \KwTo $N$ \KwBy $1$}{
Ground Plane Segmentation of $C_i$ \label{icp:ln3} 

Ground Plane Alignment of $C_i$ and $C_1$ \label{icp:ln4} 

Position Alignment of $C_i$ and $C_1$ with the known distance $d_i$ \label{icp:ln5} 

Yaw Estimation of $C_i$. \label{icp:ln6} 

% Iterative Closest Point with the previous alignment as the initial guess
}
\caption{Robust Initial Guesses Estimation for Point Clouds Alignment}
\label{algo:icp}
\end{algorithm}

\parab{Estimating Yaw.}
To estimate yaw, we leverage the following observation: for a correct estimation of the yaw angles, the closest/corresponding points between two point clouds will be coplanar \ie they should have the same normal. To this, we define the following error function:  
\begin{equation}
    E(\omega, \omega') = \Sigma_{i=1}^{n} (\perp\mathbf{R}_{\omega} p_i) \cdot (\perp\mathbf{R}_{\omega'}  q_i)
\end{equation}
where $p_i$ is a random point in the source cloud $C_1$, $q_i$ is $p_i$'s nearest neighbor in the target cloud (say $C_2$) and $n$ is the number of points in the source cloud. $\omega$ and $\omega'$ are the respective yaw angles estimates and $\mathbf{R}_\omega$ is the rotational matrix for an yaw angle of $\omega$.  $\perp$ symbolizes the normal vector estimates at a given point, say $p_i$.
With this error function, the estimation of the yaw angles can be formulated as the following optimization problem:
\begin{equation}
    Yaw_1, Yaw_2 = \argmin_{\omega,\omega'} E(\omega, \omega')
\end{equation}

We have found that ICP is robust to initial guesses for yaw that are within about 15-20$^\circ$ of the actual yaw, so \sysname discretizes the search space by this amount and performs a grid search over our defined error function (\algolineref{algo:icp}{icp:ln6}).

\section{GPU Accelerated ICP}
\label{s:gpu-accelerated-icp}

\parab{Problem.} We find that ICP is one of the main bottlenecks in \sysname's real-time processing pipeline. PCL's ICP 
implementation with the maximum number of iteration of 100 takes about 177~ms to register a point cloud of 1500 points to another point cloud of 1500 points; this exceeds \sysname's latency requirement. To optimize, we can relax the stopping criteria and allow the ICP to exit preemptively; this reduces the latency but severely compromises the accuracy. 

\parab{Proposed Solution.} The recent advancements in Graphics Processing Unit (GPU) enables fast computation of a large amount of data. \sysname exploits the parallelizable structure of ICP and uses GPU to accelerate the ICP computation while maintaining the same level of accuracy as the PCL's CPU  based ICP implementation. Table \ref{tab:icp_time_compare} shows that \sysname ICP implementation is about $60-70\times$ faster than PCL ICP implementation.

% Parallel reduction kernel. Brute force but fast.

Below, we detail the contrast between the PCL's ICP implementation with our GPU-based ICP implementation written in CUDA. In brief, PCL's ICP implementation operates via the following four steps: (1) Correspondence estimation between the source point cloud and the target point cloud, (2) Transformation estimation between source and target cloud, (3) Transformation of the source cloud by the estimated transformation matrix, and (4) Checking for the ICP convergence; we detail how we optimize each of these steps below.

\begin{table}[h]
\begin{small}
\caption{Average ICP alignment time per frame.}

\resizebox{\linewidth}{!}{
\begin{tabular}{|l|l|l|l|}
\hline
& Benchmark 1 & Benchmark 2 & Benchmark 3 \\ \hline
PCL's CPU based ICP & 177.66 ms   & 256.57 ms   & 70.93 ms \\ \hline
\begin{tabular}[c]{@{}l@{}}\sysname\\ (PCL's GPU Octree)\end{tabular} & 10.25 ms    & 11.85 ms    & 4.27 ms     \\ \hline
\sysname & 3.33 ms     & 4.27 ms     & 1.35 ms \\ \hline
\end{tabular}}
\label{tab:icp_time_compare}
\end{small}
\end{table}
\parae{Correspondence estimation.} For each point in the source cloud, correspondence estimation finds the corresponding point in the target point cloud. The correspondence estimation in ICP is achieved by nearest neighbor search: for each point $p$ in the source cloud, ICP identifies the nearest point in the target cloud $q$. Our first cut of a GPU-based ICP utilizes PCL's GPU implementation of Octree to implement the nearest neighbor search. However, due to the iterative searching in an octree, we are unable to take advantage of parallelization which again became a bottleneck. Instead, we implement a new version to leverage the parallelizable nature of the nearest neighbor search algorithm. To this, \sysname, first, applies a parallel brute-force distance calculation method (proposed in \cite{garcia2008fast}) to calculate a pairwise distance matrix. Next, \sysname leverages a modified version of insertion sort (\cite{garcia2008fast}) to find the nearest neighbor for each query point based on the calculated distance matrix. However, the modified insertion sort in \cite{garcia2008fast} applies a linear reduction in CUDA kernel and scans through each row of the distance matrix to find the nearest neighbor; this scan can be optimized further by parallelizing the scans across the rows. \sysname employs CUDA's parallel reduction functionality to implement such parallel scanning; this reduces the ICP runtime.

% However, \cite{garcia2008fast} uses a modified insertion sort to find the nearest neighbor for each query point based on the distance matrix. The modified insertion sort is a linear reduction CUDA kernel that scans through each row of the distance matrix to find the nearest neighbor, and the scan is not parallelizable within each row(but parallelizable across rows). Instead, \sysname further optimizes the nearest neighbor searching by employing CUDA's parallel reduction functionality that enables parallel searches for the nearest neighbor in each row.

\parae{Transformation estimation.} In this step, ICP utilizes the available point correspondences information to estimate the transformation matrix.  To this, PCL's ICP implementation, first, \textit{shuffles} the points in the target point cloud such that the corresponding points have the same index in both source and target points arrays; this \textit{shuffling} is highly parallelizable. Next, it applies uses the Eigen Library's Umeyama function to calculate the transformation matrix~\cite{pcl_umeyama} ; this includes a \textit{demean operation} (subtraction of the centroid from both source and target cloud), a \textit{matrix multiplication}, and a \textit{SVD operation}. \sysname optimizes these steps by (1) parallelizing the \textit{shuffle} operation via CUDA kernels, and (2) implementing the Umeyma algorithm~\cite{umeyama} with CUDA demean kernel, cuBLAS matrix multiplication, and fast CUDA SVD computation~\cite{gao2018gpu}. 

\parae{Point cloud transformation.} The third step of each iteration of ICP is to transform the source point cloud by applying the estimated transformation matrix. PCL's ICP applies such transformation to each point of a point cloud in an iterative manner; we develop a CUDA kernel for \sysname to parallelize this process.

\parae{Convergence checking.} In the last step, ICP checks for convergence to terminate the iterative process. To this, \sysname adopt the same heuristic as PCL's ICP. However, \sysname uses a CUDA kernel and parallel reductions to calculate the Mean Squared Error(MSE) between the transformed sourced cloud and the target cloud.

\section{Centralized Planner}
\label{s:centralized-planner}

\begin{algorithm}[t]
  \caption{Centralized Planner}
  \label{algo:controller}
\SetKwFunction{CalculateDrivableSpace}{CalculateDrivableSpace}
\SetKwFunction{QueryPerception}{QueryPerception}
\SetKwFunction{MotionEstimation}{MotionEstimation}
\SetKwFunction{MotionAdaptiveBuffer}{MotionAdaptiveBuffer}
\SetKwFunction{AddDynamicObstacles}{AddDynamicObstacles}
\SetKwFunction{SippPlanning}{SippPlanning}
\SetKwFunction{RecoveryMode}{RecoveryMode}
\SetKwFunction{AddStaticObstacles}{AddStaticObstacles}
\SetKwFunction{GenerateIntervals}{GenerateIntervals}
\SetKwFunction{PriorityFunction}{PriorityFunction}
\SetKwFunction{Append}{Append}
\SetKwFunction{SendOverNetwork}{SendOverNetwork}
\SetKwInOut{Input}{Input}
\SetKwInOut{Output}{Output}

\Input{\sysname-compatible objects $V_{C}$ \\ Non-compatible objects $V_{E}$ \\ Stitched point cloud $S$}
\Output{Vehicle trajectories $W$ for $V_{C}$}
\BlankLine
$P_{C}, M_{C}, B_{C} \leftarrow $ \QueryPerception ( $V_{C}$ ) \label{c:ln1} \\ % Query perception for ego-vehicles
$P_{E}, M_{E}, B_{E} \leftarrow $ \QueryPerception ( $V_{E}$ ) \label{c:ln2} \\ % Query perception for non-ego vehicles
$S_{D} \leftarrow $ \CalculateDrivableSpace {$S$} \label{c:ln3}\\
$C. $ \AddStaticObstacles { $S_{D}$ }  \label{c:ln4}\\
% \ForEach { $v_{i}$ in $V_{E}$, $p_{i}$ in $P_{E}$, $m_{i}$ in $M_{E}$, $b_{i}$ in $B_{E}$ }
\ForEach { $v_{i}$ in $V_{E}$ } %, $p_{i}$ in $P_{E}$, $m_{i}$ in $M_{E}$, $b_{i}$ in $B_{E}$ }
{\label{c:ln5}
    $t_{i} \leftarrow$ \MotionEstimation { $p_{i}$, $m_{i}$ }  \label{c:ln6}\\
    $d_{i} \leftarrow$ \MotionAdaptiveBuffer { $t_{i}$, $b_{i}$, $m_{i}$ }\label{c:ln7} \\
    $C. $\AddDynamicObstacles { $d_{i}$ } \label{c:ln8}\\
} \label{c:ln9}
% $C. $\GenerateIntervals { } \\
$V^{'}_{C} \leftarrow $ \PriorityFunction { $V_{C}$ } \label{c:ln10}\\
\ForEach { $v_{i}$ in $V^{'}_{C}$ } %, $p_{i}$ in $P_{E}$, $m_{i}$ in $M_{E}$, $b_{i}$ in $B_{E}$ }
{\label{c:ln11}
    $w_{i} \leftarrow$ $C .$\SippPlanning { $p_{i}$, $g_{i}$ } \label{c:ln12}\\
    % $W .$\Append{ $w_{i}$ } \\
    \SendOverNetwork { $v_{i}$ , $w_{i}$ } \label{c:ln13}\\
    $d_{i} \leftarrow$ $C .$\MotionAdaptiveBuffer { $w_{i}$ } \label{c:ln14}\\
    $C. $\AddDynamicObstacles { $d_{i}$ } \label{c:ln15}\\
    % $d_{i} \leftarrow$ \MotionAdaptiveBuffer { $t_{i}$, $b_{i}$, $m_{i}$ } \\
    % $C. $\LoadDynamicObstacle { $d_{i}$ } \\
}\label{c:ln16}
\end{algorithm}

The centralized planner, which resides at the edge, takes perception data and uses it to plan paths for all \sysname-compatible vehicles. It then sends these paths to all vehicles over the network. The planner generates paths for every vehicle at 10~Hz. The local low-level controllers on-board every vehicle convert these paths to control signals (steer, throttle, and brake) that the vehicle can understand.

% \sysname uses the real-time scene understanding from the perception module to plan safe and efficient paths for \sysname-compatible vehicles. We call this component the \textit{centralized controller}. This component runs at the edge. 
%The edge runs trajectory planning for all \sysname-compatible vehicles on the road. 
% Self-driving vehicles today have a similar component today, however, this component is decentralized component so it plans a trajectory for a single vehicle. 

The perception module sends perception data about dynamic and static objects to the centralized planner. Dynamic objects include \sysname-compatible objects (vehicles with \sysname's low-level controller) and non-compatible objects (vehicles without \sysname's low-level controller, cyclists, and pedestrians \etc). The centralized planner receives the position, bounding box, and motion vector (\algolinesref{algo:controller}{c:ln1}{c:ln2}) of every dynamic object from the perception module. Static objects include drivable area, the sidewalk, buildings, and traffic lights \etc For this, the planner receives a stitched 3D point cloud $S$ of the scene. It uses this to divide the scene into static obstacles and drivable space (\algolineref{algo:controller}{c:ln3}).

The planner uses SIPP to plan every \sysname-compatible vehicle's motion. The planner converts the stitched point cloud $S$ into a 2D occupancy grid $S_{D}$ (with drivable and non-drivable blocks) and feeds it to SIPP (\algolinesref{algo:controller}{c:ln3}{c:ln4}). In a single agent scenario \ie only a single vehicle with no dynamic object, this occupancy grid would be enough for SIPP to plan a collision-free path. But in a realistic scenario, dynamic obstacles include both \sysname-compatible and non-compatible objects. \sysname needs to make SIPP aware of the locations of the objects at every instant in time to plan collision-free paths. \sysname knows paths for all compatible objects because it plans paths for them. However, it has no way of knowing trajectories for non-compatible objects.

% an   The inputs to SIPP are: a) source and destination locations of the agent/car, and b) the set of obstacles in the environment. The set of obstacles consist of persistent static obstacles \eg the side-walk or a building and dynamic obstacles \eg traffic participants like other vehicles and pedestrains. Using these, SIPP plans the shortest non-collision path for the vehicle from source to destination.

To surmount this challenge, \sysname estimates the motion of all non-compatible vehicles\footnote{Like vehicles, we can estimate the motion of pedestrians as well. In this paper, we focus only on vehicles and the extension to pedestrians for future work.} and then feeds these estimates to SIPP (\algolinesref{algo:controller}{c:ln5}{c:ln9}). To do motion estimation for a non-compatible vehicle $v_{i}$, \sysname uses its motion vector $m_{i}$ and position estimate $p_{i}$ to forecast its trajectory $t_{i}$ over the next $X$ steps. To incorporate the vehicle's actual dimensions, \sysname uses the bounding boxes of every vehicle. However, this is not enough to relax the instant start/stop assumption of the SIPP algorithm or compensate for errors in perception/motion estimation.

To help alleviate the instant start/stop assumption and make the planner robust to perception errors, we form a motion-adaptive buffer $d_{i}$ around the vehicle's trajectory $t_{i}$ (\algolineref{algo:controller}{c:ln7}). The motion adaptive buffer wraps a dynamic bounding box around every position of the estimated trajectory $t_{i}$ for the vehicle $v_{i}$. The dynamic bounding box ensures the safe driving distance between that vehicle and \sysname-compatible vehicles. This dynamic bounding box is a function of the vehicle bounding box $b_{i}$ and its motion vector $m_{i}$. At rest, the dynamic bounding box is the smallest and grows as the vehicle moves faster. Then, the planner feeds this to SIPP as a dynamic obstacle (\algolineref{algo:controller}{c:ln8}). The planner uses the same technique for all non-compatible vehicles $V_{E}$ as well. 
% Finally, the controller combines the motion-adaptive buffered trajectories of all vehicles and 

Next, the planner plans paths for all \sysname-compatible vehicles sequentially. The sequential order in which paths are planned allows for user-defined traffic policies. For instance, to prioritize an emergency vehicle at an intersection, SIPP will plan for it first and then use it as a dynamic obstacle for all other vehicles. So, the planner sorts \sysname-compatible vehicles $V^{'}_{C}$ based on a user-defined policy (\algolineref{algo:controller}{c:ln10}). After this, the planner feeds the current position $p_{i}$ and goal $g_{i}$ of every compatible vehicle $v_{i}$ to SIPP. SIPP generates a set of collision-free way-points $w_{i}$ to take the vehicle from it position $p_{i}$ to its destination $g_{i}$ (\algolineref{algo:controller}{c:ln12}). The planner sends these set of waypoints to the vehicle's onboard local low-level control module over the network (\algolineref{algo:controller}{c:ln13}) using their cyber-physical association. Like a non-compatible vehicle, the planner forms a motion-adaptive buffer around the current vehicle's trajectory and feeds it to SIPP as a dynamic obstacle for the next vehicle (\algolinesref{algo:controller}{c:ln14}{c:ln15}). In the end, the planner plans and sends paths to all compatible vehicles.

\section{Local Controller}
\label{s:local-controller}

Every \sysname-compatible vehicle has an on-board local low-level controller and PID controller that receives the set of planned way-points from the centralized planner over the network (\algoref{algo:planner}). The local controller translates these to low-level control signals (throttle, steer, and brake) that can be directly applied to each vehicle. The local controller runs every 2-3~ms in the vehicle. 

The local controller receives the planned trajectory $w$ from the centralized planner every 100~ms (\algolineref{algo:planner}{p:ln1}). The planner may fail to plan a path for a vehicle or there might be a network failure. For robustness, the low-level controller checks if it has received the trajectory within a latency budget and if the received path is valid (\algolineref{algo:planner}{p:ln2}). If either of these is not true, it goes into recovery mode (\algolineref{algo:planner}{p:ln3}). In recovery mode, the controller uses the last valid planned trajectory for the vehicle. The trajectory that the controller receives informs it of the vehicle's planned path for the next $X$ steps. It would have sufficed to send the vehicle its position for just the next 100~ms but this redundancy helps relax SIPP's instant start/stop assumption and introduces robustness.

%\ramesh{The previous paragraph is important from a networking perspective. This idea is similar to soft state that permits robustness; see the Clark paper in the 551 readings.}

Given the planned trajectory $w$, the controller determines whether the vehicle has to wait at any point along its path (\algolineref{algo:planner}{p:ln5}). We call this the wait cycle. If there is a wait cycle, it finds the position $p_{s}$ associated with the wait cycle and the distance of the vehicle from it $d_{s}$ (\algolineref{algo:planner}{p:ln6}). Next, the controller calculates the braking distance $d_{b}$ (distance to bring the vehicle to a stop) of the vehicle using its current velocity $v$ (\algolineref{algo:planner}{p:ln7}). If the braking distance is less than or equal to the distance from the stopping point (\algolineref{algo:planner}{p:ln8}), the controller generates a signal $S$ to apply brakes (\algolineref{algo:planner}{p:ln9}). Without this, vehicles would apply brakes at the spatial position of the wait cycle and hence overshoot it. With this maneuver, \sysname ensures that vehicles can adhere to SIPP's collision-free planned paths. On the other hand, if the vehicle is far away from the stopping point, then the controller generates a signal $S$ to continue moving the vehicle towards the stopping point (\algolineref{algo:planner}{p:ln11}). We calculate braking distance using a standard equation~\cite{brakingdistance}.% and multiply it with a safety factor for robustness.

%\ramesh{I couldn't find where wait cycle was previously defined.}
%\fawad{Addressed.}

If there is no wait cycle in the entire trajectory $w$, the controller selects the next suitable way-point $p$ (\algolineref{algo:planner}{p:ln14}) and generates a signal to move the vehicle towards that way-point (\algolineref{algo:planner}{p:ln15}). Finally, the local controller applies the control signal $S$ to the vehicle (\algolineref{algo:planner}{p:ln17}).

\begin{algorithm}[t]
  \caption{Local Controller}
  \label{algo:planner}
\SetKwFunction{ReceiveTrajectory}{ReceiveTrajectory}
\SetKwFunction{ValidControlCycle}{ValidControlCycle}
\SetKwFunction{ValidTrajectory}{ValidTrajectory}
\SetKwFunction{RecoveryMode}{RecoveryMode}
\SetKwFunction{HasWaitCycle}{HasWaitCycle}
\SetKwFunction{GetWaitPoint}{GetWaitPoint}
\SetKwFunction{GetBrakingDistance}{GetBrakingDistance}
\SetKwFunction{ApplyBrake}{ApplyBrake}
\SetKwFunction{MoveToWaypoint}{MoveToWaypoint}
\SetKwFunction{SelectWaypoint}{SelectWaypoint}
\SetKwFunction{ApplyControl}{ApplyControl}
\SetKwInOut{Input}{Input}
\SetKwInOut{Output}{Output}

\Input{Centralized planned trajectory $t$}
\Output{Low-level control signal $S$}
\BlankLine
$w \leftarrow$ \ReceiveTrajectory { } \label{p:ln1}\\
\If  { $!$ \ValidControlCycle {$w$}  }
     {  \label{p:ln2}
        $w \leftarrow$ \RecoveryMode { } \label{p:ln3}\\
     }\label{p:ln4}
    
\eIf { \HasWaitCycle {$w$} }
     {\label{p:ln5}
        $d_{s}, p_{s} \leftarrow$ \GetWaitPoint { $w$ } \label{p:ln6} \\
        $d_{b} \leftarrow$ \GetBrakingDistance { $v$ } \label{p:ln7}\\
        \eIf { $d_{b}$ $\leq$ $d_{s}$  }
        {\label{p:ln8}
            $S \leftarrow$ \ApplyBrake { }  \label{p:ln9}\\
        }
        {
            $S \leftarrow$ \MoveToWaypoint { $p_{s}$ } \label{p:ln11} \\
        }
     }
     {
        $p \leftarrow$ \SelectWaypoint { $w$ } \label{p:ln14}\\
        $S \leftarrow$ \MoveToWaypoint { $p$ } \label{p:ln15}\\
     }\label{p:ln16}
\ApplyControl {$S$} \label{p:ln17}\\
\end{algorithm}
